# Supplementary material for: Coordinate Ascent for Off-Policy RL with Global Convergence Guarantees
Source: arXiv:2212.05237 source file (2022-12-10)
Supplement: Supplementary file 1 [file appendix_OnPG.tex]

\section{Convergence of Stochastic Vanilla Policy Gradient}
\label{app:on_pg}
\begin{proof}
The proof follows the similar idea as the proof in \citet{mei2021understanding} Theorem 3, which shows that under stochastic NPG update, it is possible to stuck in the local optimum. However, we now extends the proof to the SPG update with no importance correction (\eqref{eq:spg_update}).
The proof consists of several steps:

%\tmp{TODO: ASSUMPTIONS HERE}
\begin{itemize}[leftmargin=*]
    \vspace{-1mm}
    \item Shows that under the above assumptions, $\operatorname{Pr}\left(\mathcal{E}_{t}\right) \geq \prod_{s=1}^{t} b_{s}$
    \vspace{-1mm}
    \item Shows that there exists a suitable choice of $b_s$ such that $\prod_{s=1}^{t} b_{s} > 0$. 
\end{itemize}
\vspace{-1mm}

Let $\mathcal{E}_{t}$ be the event that the optimal action $a^{*}$ is not sampled in the first $t$ time steps. We want to show that as $t \rightarrow \infty$, $\operatorname{Pr}\left(\mathcal{E}_{t}\right) > 0$.

When $a^{*}$ is not sampled in the first $t$ steps, we have:
\begin{align}
\theta_{t}(a) &= \theta_{1}(a) + \eta \cdot \sum_{s=1}^{t-1} \frac{d \pi_{s}^{\top} r}{d \theta_{s}(a)} \\
&= \theta_{1}(a) + \eta \cdot \sum_{s=1}^{t-1} (\mathbb{I}\left[a=a_{s}\right] - \pi_{s}(a)) \cdot r(a_{s}) \\
&\ge \theta_{1}(a) + \eta \cdot r_{min} \cdot \sum_{s=1}^{t-1} (\mathbb{I}\left[a=a_{s}\right] - \pi_{s}(a)),  \left(r_{\min }:=\min _{a \neq a^{*}} r(a)\right)
\end{align}

Since 
$\pi_{\theta_{t}}(a^{*}) = \frac{\exp \left\{\theta_{t}\left(a^{*}\right)\right\}}{\sum_{a \neq a^{*}} \exp \left\{\theta_{t}(a)\right\}+\exp \left\{\theta_{t}\left(a^{*}\right)\right\}}$
we first compute the first term of the denominator:
\begin{align}
&\sum_{a \neq a^{*}} \exp \left\{\theta_{t}(a)\right\} \geq(K-1) \cdot \exp \left\{\frac{\sum_{a \neq a^{*}} \theta_{t}(a)}{K-1}\right\} \quad \text { (by Jensen's inequality) } \\
&\quad\geq (K-1) \cdot \exp \left\{\frac{\sum_{a \neq a^{*}} \theta_{1}(a)+\eta \cdot r_{\min } \cdot \sum_{a \neq a^{*}} \sum_{s=1}^{t-1} \left(\mathbb{I}\left\{a_{s}=a\right\} - \pi_s(a)\right)}{K-1}\right\} \\
&\quad= (K-1) \cdot \exp \left\{\frac{\sum_{a \neq a^{*}} \theta_{1}(a)+\eta \cdot r_{\min } \cdot \left[(t-1) - \sum^{t-1}_{s=1}\sum_{a \neq a^{*}} \pi_s(a)\right]}{K-1}\right\} \\
&\quad= (K-1) \cdot \exp \left\{\frac{\sum_{a \neq a^{*}} \theta_{1}(a)+\eta \cdot r_{\min } \cdot \left[(t-1) - \sum^{t-1}_{s=1}\left(1 - \pi_s(a^{*})\right)\right]}{K-1}\right\} \\
%
% &\quad= (K-1) \cdot \exp \left\{\frac{\sum_{a \neq a^{*}} \theta_{1}(a)+\eta \cdot r_{\min } \cdot \left[(t-1) - \sum^{t-1}_{s=1}\left(1 - \pi_s(a^{*})\right)\right]}{K-1}\right\} \\
%
&\quad= (K-1) \cdot \exp \left\{\frac{\sum_{a \neq a^{*}} \theta_{1}(a)+\eta \cdot r_{\min } \cdot \left[ \sum^{t-1}_{s=1}\pi_s(a^{*})\right]}{K-1}\right\} \\
&\quad\geq (K-1) \cdot \exp \left\{\frac{\sum_{a \neq a^{*}} \theta_{1}(a)+\eta \cdot r_{\min } \cdot \left[ \sum^{t-1}_{s=1}\pi_t(a^{*})\right]}{K-1}\right\} \\
&\quad\geq (K-1) \cdot \exp \left\{\frac{\sum_{a \neq a^{*}} \theta_{1}(a)+\eta \cdot r_{\min } \cdot \left[ \pi_1(a^{*}) + c_{t}\right]}{K-1}\right\} \\
% &\quad \geq (K-1) \cdot \exp \left\{\frac{\sum_{a \neq a^{*}} \theta_{1}(a)+\eta \cdot r_{\min } \cdot \left[(t-1) \pi_{t}(a^*)\right]} {K-1}\right\} 
\end{align}
where we use the fact that $\sum_{a \neq a^{*}} \sum_{s=1}^{t-1} \mathbb{I}\left\{a_{s}=a\right\} = t-1$  and $\pi(a^{*}) = 1 - \sum_{a \neq a^{*}} \pi(a)$.

Note that since $a^{*}$ is not sampled for the first $t$ steps, $\theta_{t}(a^{*}) \leq \theta_{1}(a^{*})$, we have:
\begin{align}
\label{eq:sum_a_lowerbound}
&\sum_{a \neq a^{*}} \pi_{\theta_{t}}(a) = 1 - \pi_{t}(a^{*}) \\
&\quad= 1 - \frac{\exp \left\{\theta_{t}\left(a^{*}\right)\right\}}{\sum_{a \neq a^{*}} \exp \left\{\theta_{t}(a)\right\}+\exp \left\{\theta_{t}\left(a^{*}\right)\right\}} \\
&\quad\geq 1 - \frac
{\exp\left\{\theta_{t}\left(a^{*}\right)\right\}}
{\sum_{a \neq a^{*}} (K-1) \cdot \exp \left\{\frac{\sum_{a \neq a^{*}} \theta_{1}(a)+\eta \cdot r_{\min } \cdot \left[(t-1) \pi_{t}(a^*)\right]} {K-1}\right\} + \exp \left\{\theta_{t}\left(a^{*}\right)\right\}} \\
\end{align}

\begin{lemma} For all $x \in(0,1)$, we have:
\label{lemma:exp_lower_bound}
\end{lemma}
\begin{equation}
\label{eq:exp_lower_bound}
1-x \geq \exp \left\{\frac{-x}{1 - x}\right\}
\end{equation}
\begin{proof}
\begin{align}
1-x &=\exp \{\log (1-x)\} \\
& \geq \exp \left\{1-e^{-\log (1-x)}\right\} \quad\left(y \geq 1-e^{-y}\right) \\
&=\exp \left\{\frac{-1}{1 / x-1}\right\}
\\
&=\exp \left\{\frac{-x}{1 - x}\right\}
\end{align}
we can plug in $x$ as $\frac{a}{b}$ to obtain a more useful form of this lemma: 
\begin{equation}
\label{eq:exp_lower_bound2}
1 -\frac{a}{b} \ge \exp \left\{\frac{-a}{b-a} \right\}
\end{equation}
\end{proof}

Using lemma \ref{lemma:exp_lower_bound} and \eqref{eq:sum_a_lowerbound} we have:
\begin{align}
\sum_{a \neq a^{*}} \pi_{\theta_{t}}(a) &= 1 - \pi_{t}(a^{*}) \\
&\geq \exp \left\{\frac{-\exp\left\{\theta_{t}\left(a^{*}\right)\right\}}{(K-1) \cdot \exp \left\{\frac{\sum_{a \neq a^{*}} \theta_{1}(a)+\eta \cdot r_{\min } \cdot \left[(t-1) \pi_{t}(a^*)\right]} {K-1}\right\}}\right\}
\end{align}

So the probability that $a^{*}$ is not sampled in the first t steps is:
\begin{align}
\operatorname{Pr}(\mathcal{E}) &\geq \prod_{t=1}^{\infty} \exp \left\{\frac{-\exp\left\{\theta_{t}\left(a^{*}\right)\right\}}{(K-1) \cdot \exp \left\{\frac{\sum_{a \neq a^{*}} \theta_{1}(a)+\eta \cdot r_{\min } \cdot \left[(t-1) \pi_{t}(a^*)\right]} {K-1}\right\}}\right\} \\
%
% &\geq \exp\left\{ \frac{-\exp\left\{\theta_{1}\left(a^{*}\right)\right\}}{(K-1)}
% \frac{1}
% {\exp\left\{\frac{\sum_{a \neq a^{*}}  \theta_{1}(a)}{K-1}\right\}}
% \sum_{t=1}^{\infty}  \frac{1}{\exp \left\{\frac{\eta \cdot r_{\min } \cdot (t-1) \cdot \pi_{t}(a^*)} {K-1}\right\}}\right\} \\
%
&\geq \exp\left\{ \frac{-\exp\left\{\theta_{1}\left(a^{*}\right)\right\}}{(K-1)}
\frac{1}
{\exp\left\{\frac{\sum_{a \neq a^{*}}  \theta_{1}(a)}{K-1}\right\}}
\sum_{t=1}^{\infty}  \frac{1}{\exp \left\{\frac{\eta \cdot r_{\min } \cdot \left(\pi_{1}\left(a^*\right) + c_{t}\right)} {K-1}\right\}}\right\} 
\end{align}

\end{proof}
